# Supplementary material for: Multimodal Agricultural Agent Architecture (MA3): A New Paradigm for Intelligent Agricultural Decision-Making
Source: arXiv:2504.04789 source file (2025-04-07)
Supplement: Supplementary file 1 [file loss.tex]

\section{Loss}
The Hungarian loss function $\mathcal{L}_{\text{Hungarian}}(y, \hat{y})$ is defined as follows:
\begin{align*}
\mathcal{L}_{\text{Hungarian}}(y, \hat{y}) &= \sum_{i=1}^N \left[ -\log \hat{p}_{\sigma(i)}(c_i) + \mathbb{1}_{\{c_i \neq \varnothing\}} \mathcal{L}_{\text{box}}(b_i, \hat{b}_{\sigma(i)}) \right] \\
\mathcal{L}_{\text{box}}(b_i, \hat{b}_{\sigma(i)}) &= \lambda_{\text{L1}} \| b_i - \hat{b}_{\sigma(i)} \|_1 + \lambda_{\text{IoU}} \mathcal{L}_{\text{IoU}}(b_i, \hat{b}_{\sigma(i)})
\end{align*}

% \begin{align*}
% \mathcal{L}_{\text{Hungarian}}(y, \hat{y}) &= \sum_{i=1}^N \left[ -\log \hat{p}_{\sigma(i)}(c_i) + \text{1}_{\{c_i \neq \varnothing\}} \mathcal{L}_{\text{box}}(b_i, \hat{b}_{\sigma(i)}) \right] \\
% \mathcal{L}_{\text{box}}(b_i, \hat{b}_{\sigma(i)}) &= \lambda_{\text{L1}} \| b_i - \hat{b}_{\sigma(i)} \|_1 + \lambda_{\text{ioU}} \mathcal{L}_{\text{ioU}}(b_i, \hat{b}_{\sigma(i)})
% \end{align*}
where:
\begin{itemize}
    \item $N$ is the total number of ground-truth objects.
    \item $y$ represents the ground-truth labels, and $\hat{y}$ represents the predicted labels.
    \item $c_i$ is the class label of the $i$-th ground-truth object.
    \item $\hat{p}_{\sigma(i)}(c_i)$ is the predicted probability of class $c_i$ for the $i$-th predicted object.
    \item $\sigma(i)$ is the index of the predicted object that matches the $i$-th ground-truth object according to the Hungarian algorithm.
    \item $\text{1}_{\{c_i \neq \varnothing\}}$ is an indicator function that equals 1 if the ground-truth class label $c_i$ is not the background class (i.e., not empty), and 0 otherwise.
    \item $\mathcal{L}_{\text{box}}(b_i, \hat{b}_{\sigma(i)})$ is the bounding box regression loss.
    \item $b_i$ and $\hat{b}_{\sigma(i)}$ are the ground-truth and predicted bounding boxes for the $i$-th object, respectively.
    \item $\lambda_{\text{L1}}$ and $\lambda_{\text{IoU}}$ are hyperparameters that balance the contributions of the L1 loss and the IoU loss, respectively.
    \item $\| b_i - \hat{b}_{\sigma(i)} \|_1$ is the L1 loss between the ground-truth and predicted bounding boxes.
    \item $\mathcal{L}_{\text{IoU}}(b_i, \hat{b}_{\sigma(i)})$ is the IoU loss between the ground-truth and predicted bounding boxes.
\end{itemize}
